# Supplementary material for: Deep Virtual Stereo Odometry: Leveraging Deep Depth Prediction for Monocular Direct Sparse Odometry
Source: arXiv:1807.02570 source file (2018-07-25)
Supplement: Supplementary file 1 [file sup_mat.tex]

% !TeX root = ../main.tex
% Add the above to each chapter to make compiling the PDF easier in some 
%editors.

\subsection{Supplementary Materials}

\begin{figure}[tbh]
	\centering
		\includegraphics[width=\textwidth]{figures/ch06/depths/stack/recons_err}
	\caption{\todo{Move this figure to somewhere in Sec.2}Image reconstruction error of SimpleNet and 
	StackNet. Both results 
		are not post-processed. The 
		disparity map predicted by StackNet shows less artifacts and the 
		reconstruction error for thin structures is reduced by the stacked 
		architecture.}
	\label{fig:stack}
\end{figure}

\begin{figure}
	{\setlength{\tabcolsep}{0.1em}
		\begin{tabular}{cccc}
			\rotatebox{90}{\tiny \ \ \ \ \ \ 
				\ \ Input} &
			
			\includegraphics[width=0.33\textwidth]{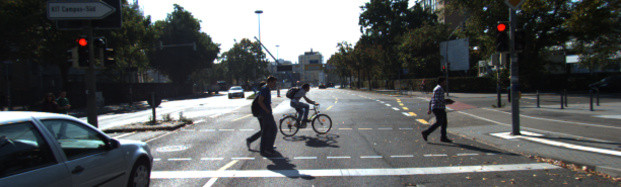}&
			
			\includegraphics[width=0.33\textwidth]{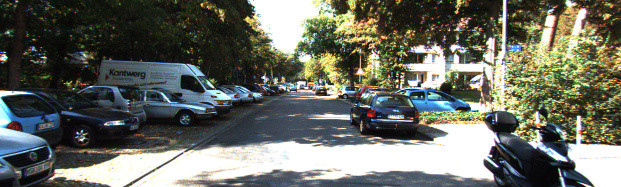}&
			
			\includegraphics[width=0.33\textwidth]{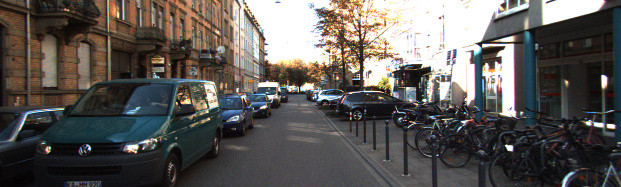}\\
			\rotatebox{90}{\tiny \ \ \ \ \ \ 
				\ GT} &
			
			\includegraphics[width=0.33\textwidth]{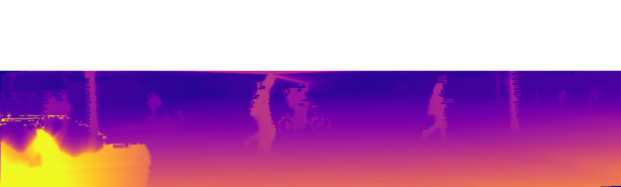}&
			
			\includegraphics[width=0.33\textwidth]{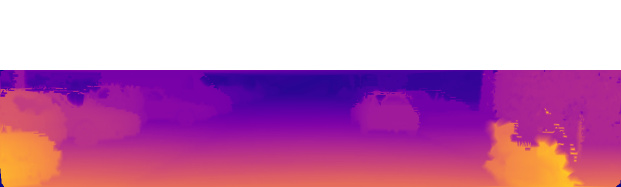}&
			
			\includegraphics[width=0.33\textwidth]{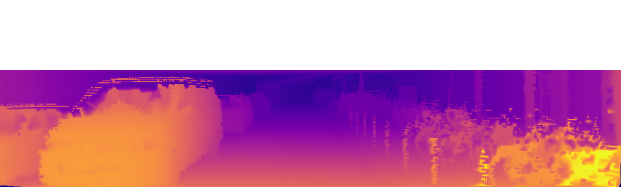}\\
			\rotatebox{90}{\tiny \ \ \ \ \ \ 
				\ Ours} &
			
			\includegraphics[width=0.33\textwidth]{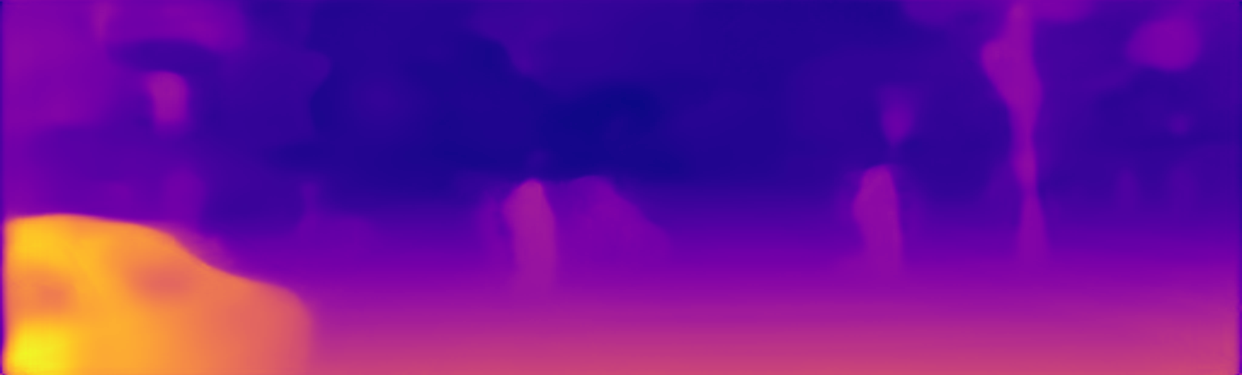}&
			
			\includegraphics[width=0.33\textwidth]{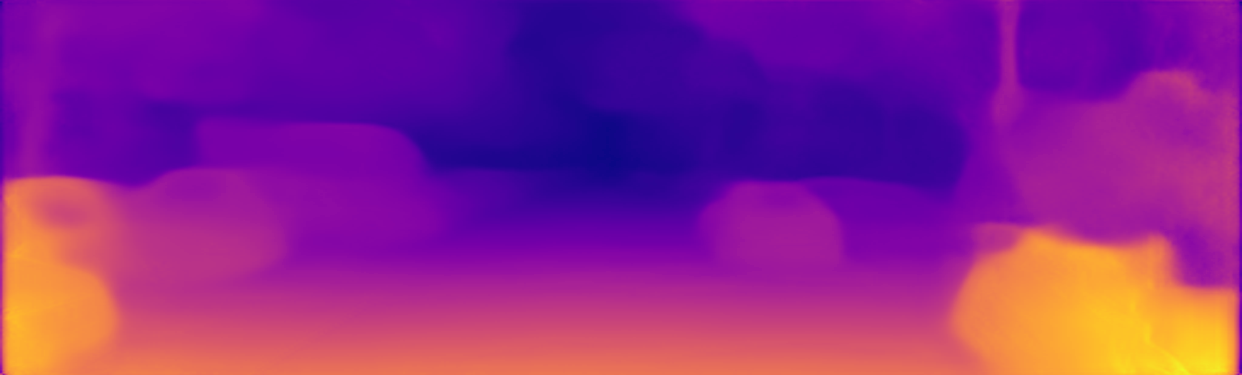}&
			
			\includegraphics[width=0.33\textwidth]{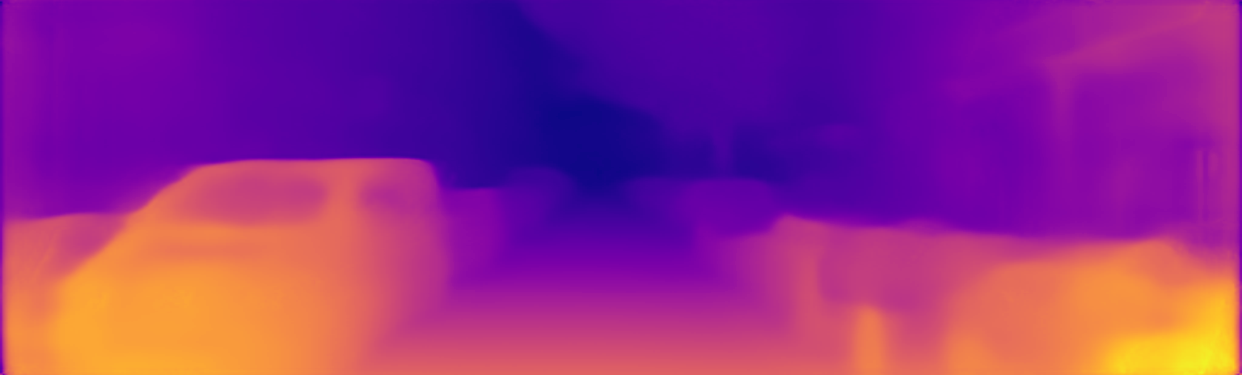}\\
			\rotatebox{90}{\tiny Kuznietsov 
				et al.~\cite{kuznietsov2017semi}} &
			
			\includegraphics[width=0.33\textwidth]{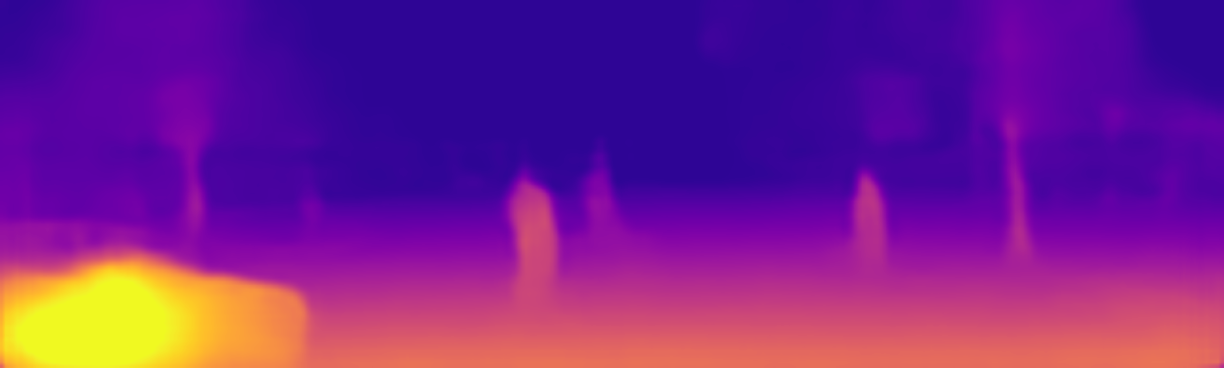}&
			
			\includegraphics[width=0.33\textwidth]{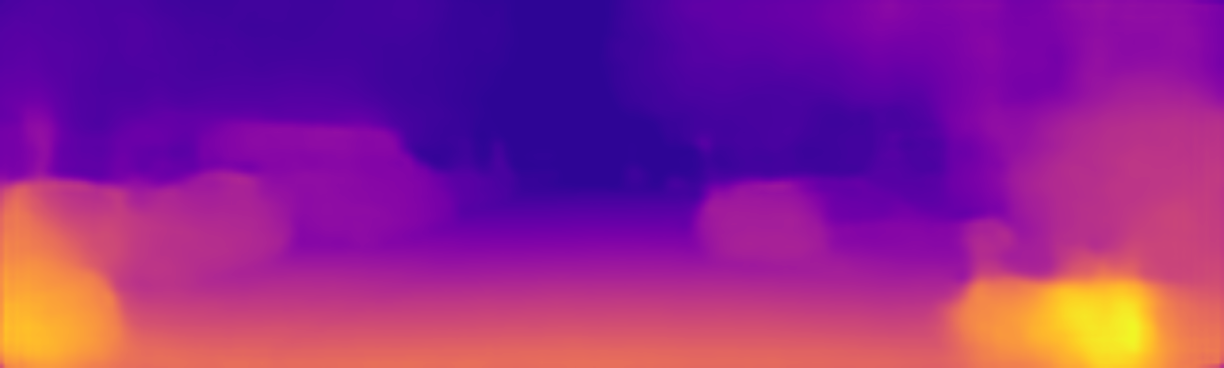}&
			
			\includegraphics[width=0.33\textwidth]{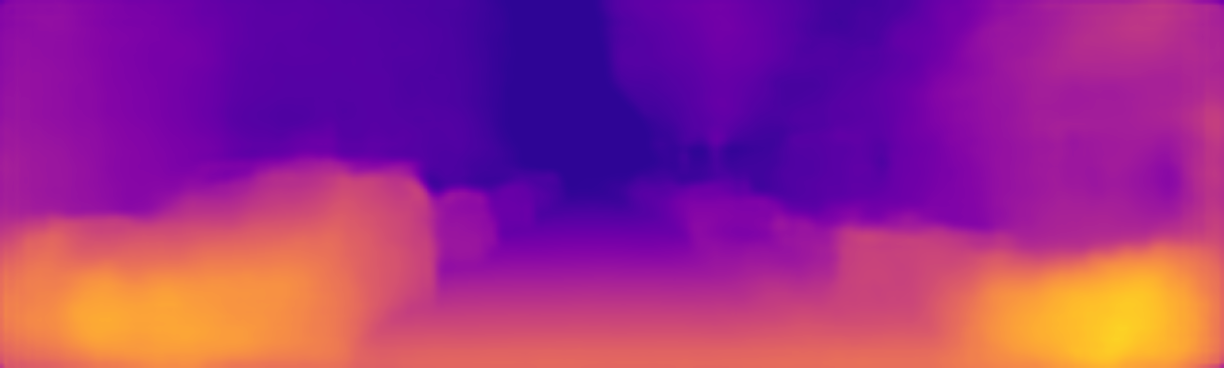}\\
			\rotatebox{90}{\tiny Godard et 
				al.~\cite{godard2016unsupervised}} &
			
			\includegraphics[width=0.33\textwidth]{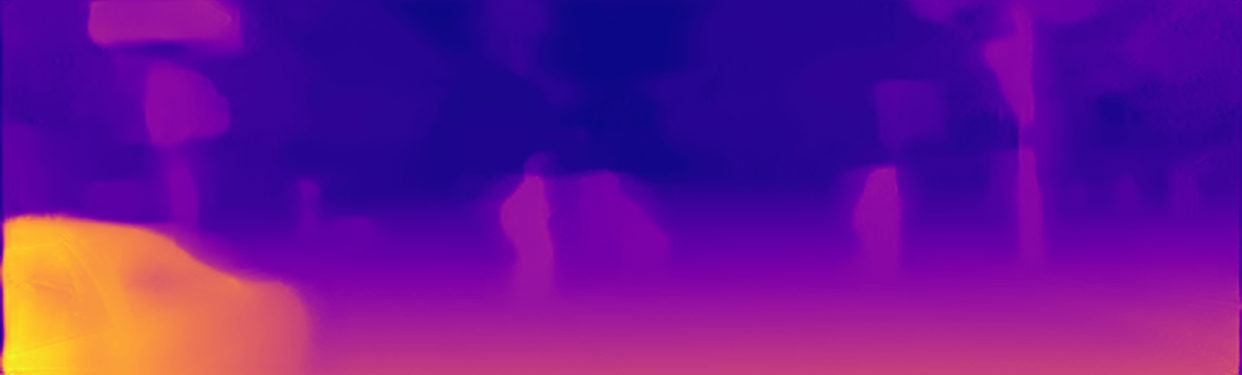}&
			
			\includegraphics[width=0.33\textwidth]{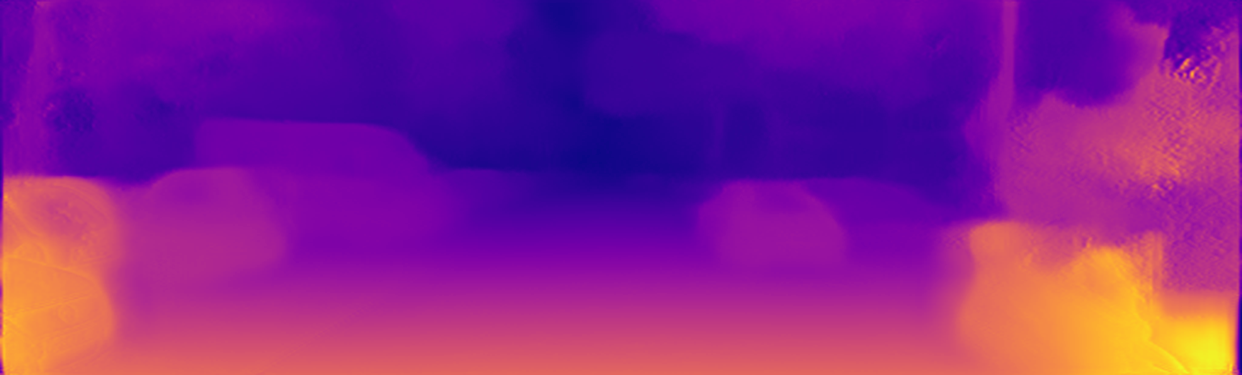}&
			
			\includegraphics[width=0.33\textwidth]{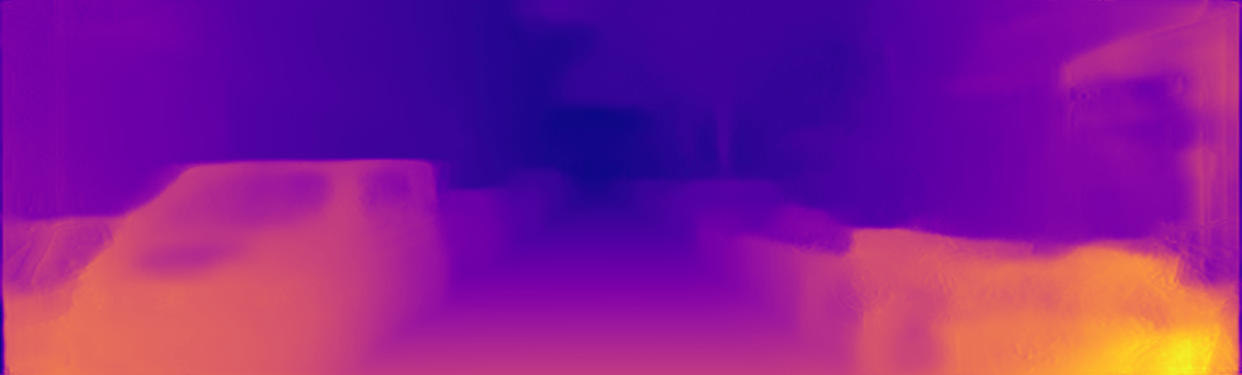}\\
			
			\rotatebox{90}{\tiny \ \ Liu et 
				al.~\cite{liu2016learning}} &
			
			\includegraphics[width=0.33\textwidth]{figures/ch06/depths/00/Liu}&
			
			\includegraphics[width=0.33\textwidth]{figures/ch06/depths/01/Liu}&
			
			\includegraphics[width=0.33\textwidth]{figures/ch06/depths/02/Liu}\\
			\rotatebox{90}{\tiny Garg et 
				al.~\cite{garg2016unsupervised}} &
			
			\includegraphics[width=0.33\textwidth]{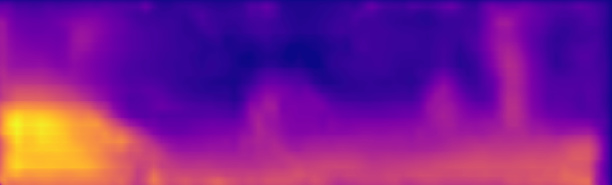}&
			
			\includegraphics[width=0.33\textwidth]{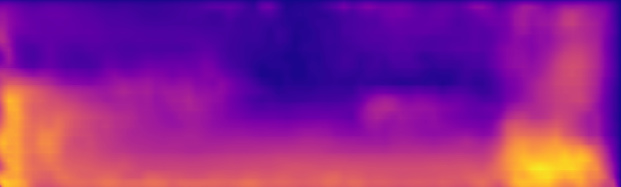}&
			
			\includegraphics[width=0.33\textwidth]{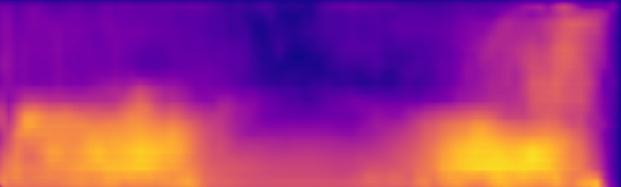}\\
			\rotatebox{90}{\tiny Eigen et 
				al.~\cite{eigen2014depth}} &
			
			\includegraphics[width=0.33\textwidth]{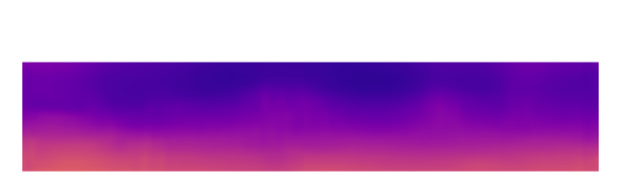}&
			
			\includegraphics[width=0.33\textwidth]{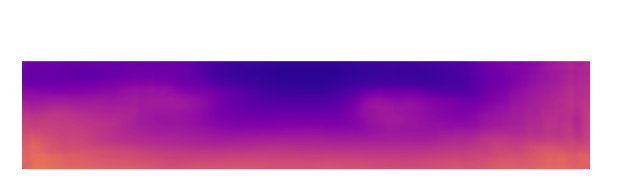}&
			
			\includegraphics[width=0.33\textwidth]{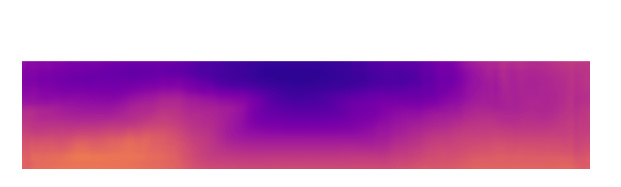}\\
		\end{tabular}
	}
	\caption{\textcolor{red}{\textbf{Do we really need to show all the 
				results of other methods?}}Qualitative comparison with 
		state-of-the-art methods. The ground 
		truth is interpolated for better visualization. Our approach shows 
		better 
		prediction on thin structures than unsupervised 
		approach\cite{godard2016unsupervised}, and delivers more detailed 
		disparity map 
		than the semi-supervised approach using LiDAR 
		data~\cite{kuznietsov2017semi}.}
	\label{fig:compare_all}
\end{figure}

\begin{figure}[ht!]
	\centering
	\begin{subfigure}[t]{.11\textwidth}
		\centering
		\includegraphics[width=\textwidth]{figures/ch06/depths/make3D/img_from_kuz/00_resize}
	\end{subfigure}
	\begin{subfigure}[t]{.11\textwidth}
		\centering
		\includegraphics[width=\textwidth]{figures/ch06/depths/make3D/img_from_kuz/kuz/00_resize}
	\end{subfigure}
	\begin{subfigure}[t]{.11\textwidth}
		\centering
		\includegraphics[width=\textwidth]{figures/ch06/depths/make3D/img_from_kuz/godard/00_resize}
	\end{subfigure}
	\begin{subfigure}[t]{.11\textwidth}
		\centering
		\includegraphics[width=\textwidth]{figures/ch06/depths/make3D/img_from_kuz/ours/00_resize}
	\end{subfigure}
	\begin{subfigure}[t]{.11\textwidth}
		\centering
		\includegraphics[width=\textwidth]{figures/ch06/depths/make3D/img_from_kuz/01_resize}
	\end{subfigure}
	\begin{subfigure}[t]{.11\textwidth}
		\centering
		\includegraphics[width=\textwidth]{figures/ch06/depths/make3D/img_from_kuz/kuz/01_resize}
	\end{subfigure}
	\begin{subfigure}[t]{.11\textwidth}
		\centering
		\includegraphics[width=\textwidth]{figures/ch06/depths/make3D/img_from_kuz/godard/01_resize}
	\end{subfigure}
	\begin{subfigure}[t]{.11\textwidth}
		\centering
		\includegraphics[width=\textwidth]{figures/ch06/depths/make3D/img_from_kuz/ours/01_resize}
	\end{subfigure}
	\begin{subfigure}[t]{.15\textwidth}
		\centering
		\includegraphics[width=\textwidth]{figures/ch06/depths/make3D/img_from_kuz/00_crop}
	\end{subfigure}
	\begin{subfigure}[t]{.15\textwidth}
		\centering
		\includegraphics[width=\textwidth]{figures/ch06/depths/make3D/img_from_kuz/godard/00_crop}
	\end{subfigure}
	\begin{subfigure}[t]{.15\textwidth}
		\centering
		\includegraphics[width=\textwidth]{figures/ch06/depths/make3D/img_from_kuz/ours/00_crop}
	\end{subfigure}
	\begin{subfigure}[t]{.15\textwidth}
		\centering
		\includegraphics[width=\textwidth]{figures/ch06/depths/make3D/img_from_kuz/01_crop}
	\end{subfigure}
	\begin{subfigure}[t]{.15\textwidth}
		\centering
		\includegraphics[width=\textwidth]{figures/ch06/depths/make3D/img_from_kuz/godard/01_crop}
	\end{subfigure}
	\begin{subfigure}[t]{.15\textwidth}
		\centering
		\includegraphics[width=\textwidth]{figures/ch06/depths/make3D/img_from_kuz/ours/01_crop}
	\end{subfigure}
	\caption{Results on the Make3D Dataset. The top row shows the predicted 
		depth maps of Kuznietsov et al.~\cite{kuznietsov2017semi}, Godard et 
		al.~\cite{godard2016unsupervised} and ours from left to right, using 
		the 
		input images with original aspect ratio. The bottom row shows the 
		results 
		of Godard et al.~\cite{godard2016unsupervised} and ours, using the 
		inputs 
		with central crop as in~\cite{godard2016unsupervised}. }
	\label{fig:m3_compare}
\end{figure}

\begin{figure}
	{\setlength{\tabcolsep}{0.1em}
		\begin{tabular}{ccc}
			RGB&Godard et al.~\cite{godard2016unsupervised}&Ours\\
			\includegraphics[width=0.33\textwidth]{figures/ch06/depths/cs/rgb/frankfurt_000000_001160_leftImg8bit.png}&
			\includegraphics[width=0.33\textwidth]{figures/ch06/depths/cs/godard/frankfurt_000000_001160_leftImg8bit.png}&
			\includegraphics[width=0.33\textwidth]{figures/ch06/depths/cs/ours/frankfurt_000000_001160_leftImg8bit.png}\\
			\includegraphics[width=0.33\textwidth]{figures/ch06/depths/cs/rgb/frankfurt_000000_005624_leftImg8bit.png}&
			\includegraphics[width=0.33\textwidth]{figures/ch06/depths/cs/godard/frankfurt_000000_005624_leftImg8bit.png}&
			\includegraphics[width=0.33\textwidth]{figures/ch06/depths/cs/ours/frankfurt_000000_005624_leftImg8bit.png}\\
			\includegraphics[width=0.33\textwidth]{figures/ch06/depths/cs/rgb/frankfurt_000001_029203_leftImg8bit.png}&
			\includegraphics[width=0.33\textwidth]{figures/ch06/depths/cs/godard/frankfurt_000001_029203_leftImg8bit.png}&
			\includegraphics[width=0.33\textwidth]{figures/ch06/depths/cs/ours/frankfurt_000001_029203_leftImg8bit.png}\\
			\includegraphics[width=0.33\textwidth]{figures/ch06/depths/cs/rgb/frankfurt_000001_041019_leftImg8bit.png}&
			\includegraphics[width=0.33\textwidth]{figures/ch06/depths/cs/godard/frankfurt_000001_041019_leftImg8bit.png}&
			\includegraphics[width=0.33\textwidth]{figures/ch06/depths/cs/ours/frankfurt_000001_041019_leftImg8bit.png}\\
			\includegraphics[width=0.33\textwidth]{figures/ch06/depths/cs/rgb/frankfurt_000001_030680_leftImg8bit.png}&
			\includegraphics[width=0.33\textwidth]{figures/ch06/depths/cs/godard/frankfurt_000001_030680_leftImg8bit.png}&
			\includegraphics[width=0.33\textwidth]{figures/ch06/depths/cs/ours/frankfurt_000001_030680_leftImg8bit.png}\\
		\end{tabular}
	}
	\caption{\textcolor{red}{\textbf{Less images?}}Generalization to the 
		Cityscapes 
		Dataset~\cite{Cordts2016Cityscapes}. 
		The depth maps are predicted 
		from the models trained on the Eigen split of KITTI dataset. Both 
		models 
		can be 
		generalized to predict plausible depth on the unseen Cityscapes 
		Dataset, 
		while 
		our 
		model 
		delivers better prediction on thin structures and, as mentioned above, 
		less 
		shadow artifact. Note that both models are not able to predict the 
		depth 
		of 
		the right-side pedestrians on the images of the last row.} 
	%We suspect this is because in KITTI Dataset, 
	%	pedestrians rarely appear in that position of the image.}.
	\label{fig:cs_compare}
\end{figure}

\begin{figure}
	\centering
	\begin{subfigure}[t]{\textwidth}
		\centering
		\includegraphics[width=.31\textwidth]{figures/ch06/trajs/monos/00_traj}
		\includegraphics[width=.31\textwidth]{figures/ch06/trajs/monos/05_traj}
		\includegraphics[width=.31\textwidth]{figures/ch06/trajs/monos/09_traj}
	\end{subfigure}
	\begin{subfigure}[t]{\textwidth}
		\centering
		\includegraphics[width=.31\textwidth]{figures/ch06/trajs/stereos/00_traj}
		\includegraphics[width=.31\textwidth]{figures/ch06/trajs/stereos/05_traj}
		\includegraphics[width=.31\textwidth]{figures/ch06/trajs/stereos/09_traj}
	\end{subfigure}
	\caption{Estimated trajectories on KITTI sequence 00, 05 and 09. Top row 
		shows the comparisons with monocular methods that are Sim(3) aligned. 
		Bottom row shows the comparisons with stereo methods. For more 
		trajectories 
		on KITTI, please refer to our supplementary materials.}
	\label{fig:kitti_traj}
\end{figure}

\begin{figure}
	\centering
	\begin{subfigure}[t]{.4\textwidth}
		\centering
		\frame{\includegraphics[width=\textwidth]{figures/ch06/trajs/test_godard/godard.pdf}}
		\caption{Using disparity maps estimated by Godard et 
			al.~\cite{godard2016unsupervised}.}
	\end{subfigure}
	\begin{subfigure}[t]{.4\textwidth}
		\centering
		\frame{\includegraphics[width=\textwidth]{figures/ch06/trajs/test_godard/ours.pdf}}
		\caption{Using disparity maps estimated by our network.}
	\end{subfigure}
	\caption{Comparison of estimated trajectories on KITTI sequence 00 with 
		disparity maps generated 
		by our model and Godard et  al.~\cite{godard2016unsupervised}. The 
		left-bottom inset shows a close-up of the end of the trajectories, 
		where we 
		can see that the one using our prediction has smaller drift.}
	\label{fig:godard_deep_dso}
\end{figure}

\begin{figure}[ht!]
	\centering
	\begin{subfigure}[t]{.49\textwidth}
		\centering
		\includegraphics[width=\textwidth]{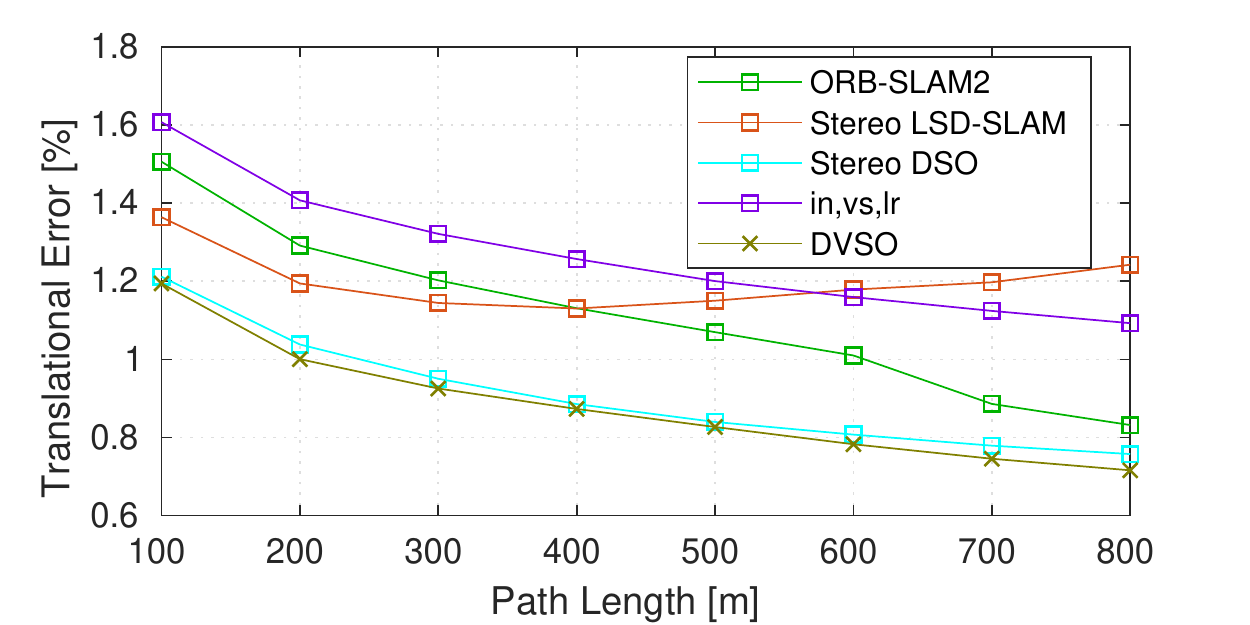}
		%		\caption{}
	\end{subfigure}
	\begin{subfigure}[t]{.49\textwidth}
		\centering
		\includegraphics[width=\textwidth]{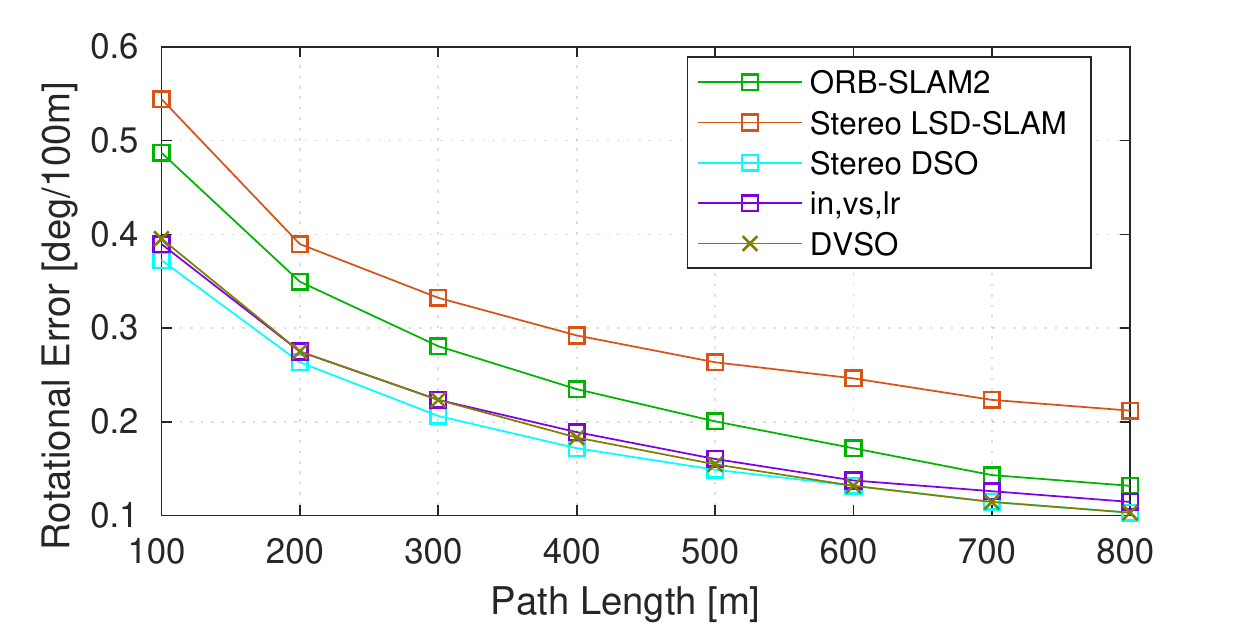}
		%		\caption{}
	\end{subfigure}
	\begin{subfigure}[t]{.49\textwidth}
		\centering
		\includegraphics[width=\textwidth]{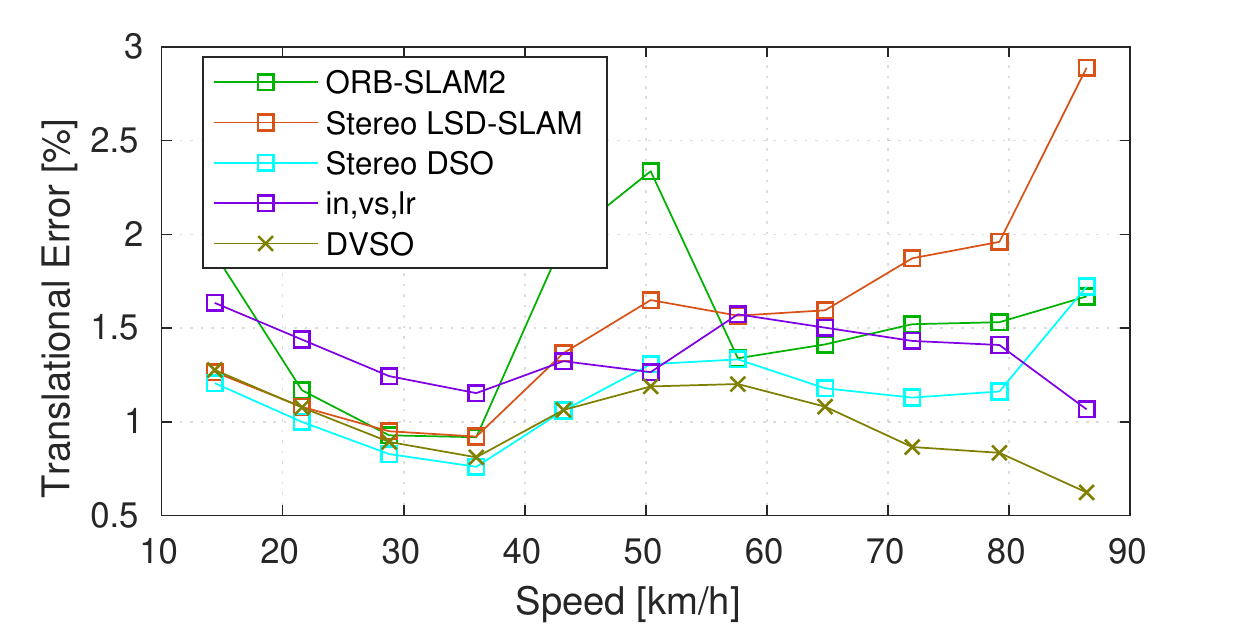}
		%		\caption{}
	\end{subfigure}
	\begin{subfigure}[t]{.49\textwidth}
		\centering
		\includegraphics[width=\textwidth]{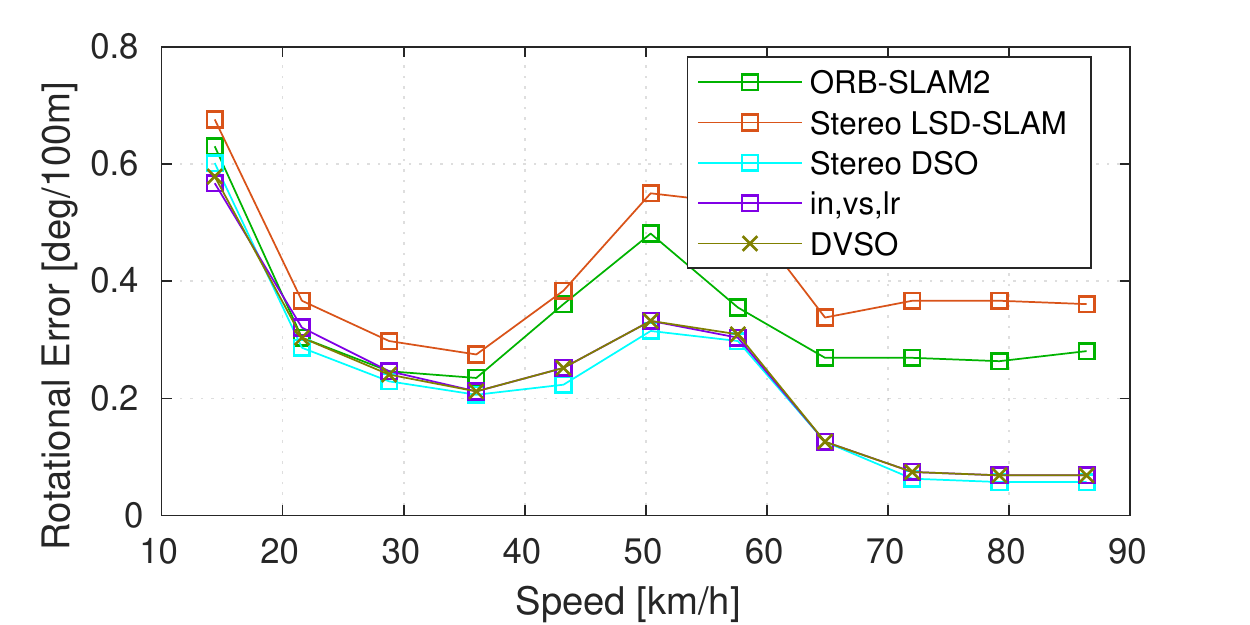}
		%		\caption{}
	\end{subfigure}
	\caption{Evaluation results on the test set of KITTI Odometry Benchmark. 
		The top row shows translational and rotational errors with respect to 
		driving 
		intervals and the bottom row shows the translational and rotational 
		errors 
		with respect to driving speed. For translational errors, DVS-DSO shows 
		comparable performance with Stereo LSD-SLAM on different path lengths, 
		while achieves better performance than Stereo LSD-SLAM on different 
		speeds. 
		For rotational errors, DVS-DSO achieves comparable results with Stereo 
		DSO 
		and better than all other methods. Note that with baseline tuning, 
		DVS-DSO$^{+}$ in general achieves the best performance among all the 
		methods evaluated.}
	\label{fig:kitti_test_set}
\end{figure}
\begin{figure}
	\centering
	\begin{subfigure}[t]{0.3\textwidth}
		\centering
		\includegraphics[width=\textwidth]{figures/ch06/trajs/cs/test_cs_0_5000.pdf}
		\caption*{Frame 0-5000}
	\end{subfigure}
	\begin{subfigure}[t]{0.3\textwidth}
		\centering
		\includegraphics[width=\textwidth]{figures/ch06/trajs/cs/test_cs_0_10000.pdf}
		\caption*{Frame 0-10000}
	\end{subfigure}
	\begin{subfigure}[t]{0.3\textwidth}
		\centering
		\includegraphics[width=\textwidth]{figures/ch06/trajs/cs/test_cs_0_15000.pdf}
		\caption*{Frame 0-15000}
	\end{subfigure}
	\begin{subfigure}[t]{0.3\textwidth}
		\centering
		\includegraphics[width=\textwidth]{figures/ch06/trajs/cs/test_cs_0_20000.pdf}
		\caption*{Frame 0-20000}
	\end{subfigure}
	\begin{subfigure}[t]{0.3\textwidth}
		\centering
		\includegraphics[width=\textwidth]{figures/ch06/trajs/cs/test_cs_0_25000.pdf}
		\caption*{Frame 0-25000}
	\end{subfigure}
	\begin{subfigure}[t]{0.3\textwidth}
		\centering
		\includegraphics[width=\textwidth]{figures/ch06/trajs/cs/test_cs_0_32000.pdf}
		\caption*{Frame 0-32000}
	\end{subfigure}
	\caption{Estimated trajectories in Cityscapes Frankfurt. The estimated 
		trajectories are Sim(3) aligned to GPS ground truth. DVS-DSO works 
		quite 
		well before 20000 frame, while the drift becomes larger afterwards.}
	\label{fig:cs_trajs}
\end{figure}
